# Supplementary material for: Dispersion relations for $\gamma^*\gamma^*\to\pi\pi$: helicity amplitudes, subtractions, and anomalous thresholds
Source: arXiv:1905.13198 source file (2019-07-16)
Supplement: Supplementary file 1 [file AppendixMOSolution.tex]

% !TEX root = ../DV_Paper.tex

\section{MO solution: coupling between $\boldsymbol{S}$- and $\boldsymbol{D}$-waves}
\label{app:MOSolution}
 
 For the $S$-waves, the non-diagonal kernel functions produce an additional inhomogeneity $\Delta(s)=\sum_{i=-1}^2 c_i s^i$. Its effect from the Cauchy kernel is
 \begin{align}
 \Delta(s)+\frac{\Omega_0(s)}{\pi}\int_{4\mpi^2}^\infty d s'\frac{\sin\delta_0(s')}{|\Omega_0(s')|}\frac{\Delta(s')}{s'-s}
 &=\Delta(s)+\sum_{i=0}^3c_{i-1} \frac{\Omega_0(s)}{\pi}\int_{4\mpi^2}^\infty d s'\frac{\sin\delta_0(s')}{|\Omega_0(s')|}\frac{s'^{i-1}}{s'-s}\notag\\
 &=\Delta(s)+\Omega_0(s)\Bigg[ \sum_{i=1}^3 c_{i-1}\bigg(-\frac{s^{i-1}}{\Omega_0(s)}\bigg) + \frac{c_{-1}}{s}\bigg(1-\frac{1}{\Omega_0(s)}\bigg)\Bigg]\notag\\
 &=c_{-1}\frac{\Omega_0(s)}{s}.
 \end{align}
 Next, the non-Cauchy kernels combine in such a way that in the sum of the two terms the $\lambda_{12}(s')$ in the denominator is canceled, leaving only $\Delta'(s)=\sum_{i=-1}^1 c_i' s^i$ in
 \begin{align}
  \frac{\Omega_0(s)}{\pi}\int_{4\mpi^2}^\infty d s'\frac{\sin\delta_0(s')}{|\Omega_0(s')|}\Delta'(s')
  &=\sum_{i=0}^2c'_{i-1} \frac{\Omega_0(s)}{\pi}\int_{4\mpi^2}^\infty d s'\frac{\sin\delta_0(s')}{|\Omega_0(s')|}s'^{i-1}\notag\\
  &=\Omega_0(s)\sum_{i=0}^2c'_{i-1}(-\delta_{i0})=-c'_{-1}\Omega_0(s).
 \end{align}
 The resulting constant in~\eqref{MO_solution_Swaves_Dwaves} are
 \begin{align}
  \alpha_{0,1}^{(-1)}%&=10\mpi^2(q_1^2-q_2^2)^2\frac{1}{\pi}\int_{4\mpi^2}^\infty\frac{d s'}{\lambda_{12}^2(s')}
%\bigg[-2q_1^2q_2^2s'\Im \tilde h_{2,5}(s')\notag\\
%&+\big(s'(q_1^2+q_2^2)-(q_1^2-q_2^2)^2\big)\Big(\Im \tilde h_{2,1}(s')-\frac{s'}{\sqrt{6}}\Im \tilde h_{2,3}(s')\Big)\notag\\
%&+\frac{s'}{\sqrt{6}}(s'-q_1^2-q_2^2)\Big(\Im \tilde h_{2,2}(s')+(q_1^2-q_2^2)^2\Im\tilde h_{2,4}(s')\Big)\bigg]\notag\\
&=5\mpi^2s_+s_-\frac{1}{\pi}\int_{4\mpi^2}^\infty\frac{d s'}{\lambda_{12}^2(s')s'}
\bigg[s_-(s'-s_+)\Im h'_2(s')+s_+(s'-s_-)\Im h'_3(s')\notag\\
&+\frac{\lambda_{12}(s')}{\sqrt{6}}\Big(2(s_++s_-)\Im h'_1(s')+(s'-s_+)\Im h'_4(s')+(s'-s_-)\Im h'_5(s')\Big)
\bigg]
,\notag\\
\alpha_{0,5}^{(-1)}%&=10\mpi^2(q_1^2-q_2^2)^2\frac{1}{\pi}\int_{4\mpi^2}^\infty\frac{d s'}{\lambda_{12}^2(s')}
%\bigg[-2s'\bigg(\Im \tilde h_{2,1}(s')+\frac{1}{\sqrt{6}}\big(\Im \tilde h_{2,2}(s')-s'\Im\tilde h_{2,3}(s')\big)\bigg)\notag\\
%&-\frac{s'}{\sqrt{6}}\big(\lambda_{12}(s')+2(q_1^2-q_2^2)^2\big)\Im \tilde h_{2,4}(s')+\big(s'(q_1^2+q_2^2)-(q_1^2-q_2^2)^2\big)\Im\tilde h_{2,5}(s')\bigg]\notag\\
&=-10\mpi^2s_+s_-\frac{1}{\pi}\int_{4\mpi^2}^\infty\frac{d s'}{\lambda_{12}^2(s')s'}
\bigg[s'(\Im h'_2(s')+\Im h'_3(s'))+\big(2s_+s_--s'(s_++s_-)\big)\Im h'_{23}(s')\notag\\
&+\frac{\lambda_{12}(s')}{\sqrt{6}}\Big(4\Im h'_1(s')-\Im h'_4(s')-\Im h'_5(s')+(2s'-s_+-s_-)\Im h'_{45}(s')\Big)\bigg],\notag\\
\alpha_{0,1}^{(0)}%&=10\mpi^2\frac{1}{\pi}\int_{4\mpi^2}^\infty\frac{d s'}{\lambda_{12}^2(s')}
%\bigg[2q_1^2q_2^2(q_1^2-q_2^2)^2\Im \tilde h_{2,5}(s')\notag\\
%&-(s'-q_1^2-q_2^2)(q_1^2-q_2^2)^2\Big(\Im \tilde h_{2,1}(s')-\frac{s'}{\sqrt{6}}\Im \tilde h_{2,3}(s')\Big)+\frac{2}{\sqrt{6}}q_1^2q_2^2s'\lambda_{12}(s')\Im\tilde h_{2,4}(s')\notag\\
%&+\frac{s'}{\sqrt{6}}\big(q_1^4+6q_1^2q_2^2+q_2^4-s'(q_1^2+q_2^2)\big)\Big(\Im \tilde h_{2,2}(s')+(q_1^2-q_2^2)^2\Im\tilde h_{2,4}(s')\Big)\bigg],\notag\\
&=-5\mpi^2\frac{1}{\pi}\int_{4\mpi^2}^\infty\frac{d s'}{\lambda_{12}^2(s')s'}
\bigg[s_+s_-\big((s'-s_+)\Im h'_2(s')+(s'-s_-)\Im h'_3(s')\big)\notag\\
&+\frac{\lambda_{12}(s')}{\sqrt{6}}\Big(4s_+s_-\Im h'_1(s')+s_-(s'-s_+)\Im h'_4(s')+s_+(s'-s_-)\Im h'_5(s')\Big)\bigg],\notag\\
\alpha_{0,5}^{(0)}%&=10\mpi^2\frac{1}{\pi}\int_{4\mpi^2}^\infty\frac{d s'}{\lambda_{12}^2(s')}
%\bigg[2(q_1^2-q_2^2)^2\Big(\Im \tilde h_{2,1}(s')-\frac{s'}{\sqrt{6}}\Im \tilde h_{2,3}(s')\Big)\notag\\
%&-\frac{2s'}{\sqrt{6}}\big(s'-2(q_1^2+q_2^2)\big)\Big(\Im \tilde h_{2,2}(s')+(q_1^2-q_2^2)^2\Im\tilde h_{2,4}(s')\Big)\notag\\
%&+\frac{s'}{\sqrt{6}}(q_1^2+q_2^2)\lambda_{12}(s')\Im\tilde h_{2,4}(s')-(s'-q_1^2-q_2^2)(q_1^2-q_2^2)^2\Im\tilde h_{2,5}(s')\bigg]\notag\\
&=-10\mpi^2\frac{1}{\pi}\int_{4\mpi^2}^\infty\frac{d s'}{\lambda_{12}^2(s')s'}
\bigg[s_+s_-(2s'-s_+-s_-)\Im h'_{23}(s')-s_+s_-(\Im h'_2(s')+\Im h'_3(s'))\notag\\
&+\frac{\lambda_{12}(s')}{\sqrt{6}}\Big(s'(\Im h'_4(s')+\Im h'_5(s'))+\big(2s_+s_--s'(s_++s_-)\big)\Im h'_{45}(s')\Big)
\bigg].
 \end{align}
